# Supplementary material for: ScreeNOT: Exact MSE-Optimal Singular Value Thresholding in Correlated Noise
Source: arXiv:2009.12297 source file (2023-03-26)
Supplement: Supplementary file 1 [file supplement.tex]

\begin{supplement} 
\stitle{Proofs and Additional Empirical Results}
\slink[doi]{COMPLETED BY THE TYPESETTER}
\sdatatype{.pdf}
\sdescription{
  To keep within the space constraints, the proofs of several technical claims are deferred to the supplementary article.
  In addition, 
  in the supplementary material 
  we provide extensive numerical experiments validating different aspects of our results under 
  various noise distributions.
%   In the supplementary material we provide two proofs omitted from the main text for
%   space considerations.   We prove 
%   Lemma~\ref{lem:crossing} and Proposition~\ref{prop:correlations}.
%  In addition, in the supplementary material 
%  we provide extensive numerical experiments validating different aspects of our results under 
%  various noise distributions.
 }
\end{supplement}
